# Supplementary material for: Phase shift in atom interferometry due to spacetime curvature
Source: arXiv:1610.03832 ancillary file (2016-10-13)
Supplement: Supplementary file 1 [file curvatureSupplemental.pdf]

# Phase shift in atom interferometry due to spacetime curvature - Supplemental Material

Peter Asenbaum,[1] Chris Overstreet,[1] Tim Kovachy,[1] Daniel D. Brown,[2] Jason M. Hogan,[1] and Mark A. Kasevich[1]

[1] *Department of Physics, Stanford University, Stanford, California 94305*

[2] *School of Physics and Astronomy, University of Birmingham, Birmingham, B15 2TT, UK*

## GRADIOMETER PHASE VS LAUNCH POSITION

We study the systematic effect of the launch position on the gradiometer phase. By changing the position of the dipole lens, we vary the launch position by $\pm 3$ mm in the $x$ (North-South) and $y$ (East-West) direction. For the data runs presented in the main text, we control the launch position to better than 1 mm to avoid a systematic error.

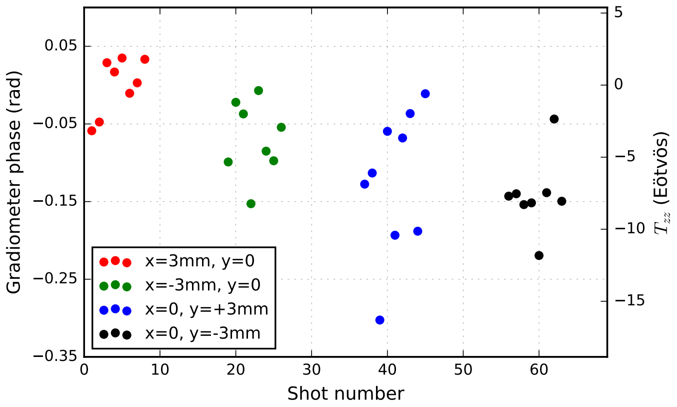


FIG. 1: Gradiometer phase for different launch positions with $h = 8.45$ m, $L = 32$ cm, $n = 20$, and $T = 600$ ms. Spread of $T_{zz}$ for the different positions: 1.8 E (red), 2.4 E (green), 4.7 E (blue), 2.4 E (black).

## PHASE SHEAR READOUT PHASE EXTRACTION

To extract the differential interferometer phase from the fluorescence images, we assume that the image of output port $i$ of an interferometer is given by

$$G_i(x, y)(1 + C_i \cos(2\pi f x + \Phi_i))/2,$$

where $G_i$ is the 2D cloud envelope, $C_i$ the output contrast, $f$ the phase shear fringe frequency, and $\Phi_i$ the interferometer phase for the $i^{\text{th}}$ port. In the least squared fitting of this model to the data, there is a strong correlation between the fringe frequency and phase. The fringe frequency is determined by the tilt of the final $\pi/2$ pulse in the interferometer and the expansion time until the cloud is imaged, which are constant from shot to shot. As the fringe frequency is assumed to be constant, it is first estimated by performing an initial run of non-linear least square fits for each shot and taking the average best fit value. A second run of fits is then performed assuming $f$ to be constant to estimate $\Phi$. This process was carried out for the two imaged ports from each interferometer, the final gradiometer phase output then being the phase difference between the two. One noticeable noise source using this method was from low spatial frequency fluctuations in the cloud shape $G_i$ from shot to shot, which coupled into noise in the estimation of $\Phi$. It was found that a high fringe frequency should be used to avoid this noise source. A typical example of how this model fits to the data is shown in Fig. 2.

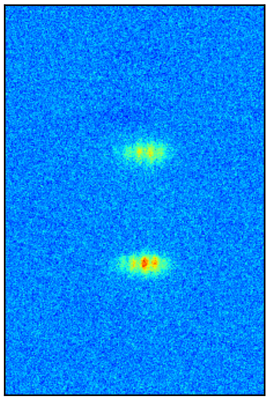

(a) Full fluorescence image including the two ports (one from each interferometer)

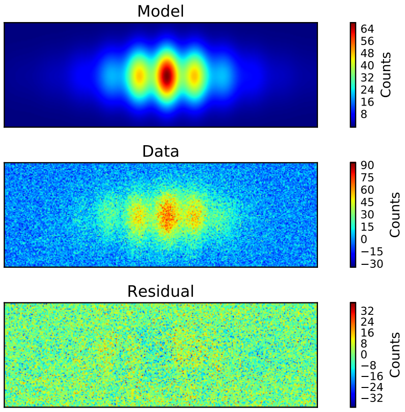


(b) Analysis of single port

FIG. 2: Typical model fit to data. Data taken from an experiment using $n = 10$ and $T = 200\,\text{ms}$, image size $1000\times666$ pixels. Shown is the analysis of a port from one of the interferometers and the best fit parameters. In this case the best fit was achieved using Gaussian shaped clouds in $x$ and $y$, and a fixed fringe wavelength of $29\,\text{px}$. The overall phase uncertainty of this shot is 21 mrad.
